# Supplementary material for: Contact Anticipation for Physical Human-Robot Interaction with Robotic Manipulators using Onboard Proximity Sensors
Source: arXiv:2110.11516 source file (2021-11-30)
Supplement: Supplementary file 1 [file appendix.tex]

\section*{APPENDIX}
